# Supplementary material for: Phenotypes of vascular flow networks
Source: arXiv:1707.03074 ancillary file (2019-12-13)
Supplement: Supplementary file 1 [file s1-appendix.pdf]

# S1 Appendix. Supplemental Material for “The Phenotypes of Fluctuating Flow: Development of Distribution Networks in Biology and the Trade-off between Efficiency, Cost, and Resilience”

Henrik Ronellenfitsch\* and Eleni Katifori†

*Department of Physics and Astronomy, University of Pennsylvania, Philadelphia, PA 19104, USA*

## I. NONDIMENSIONALIZATION OF THE MODEL

Here, we explicitly derive the nondimensionalization of the dynamical equations presented in the main paper. The dimensionful dynamical equations used in the main paper are

$$\mathbf{F}_i = K L^{-1} \Delta (\Delta^T K L^{-1} \Delta)^\dagger \mathbf{S}_i \quad (1)$$

$$\frac{dK_e}{dt} = a \left\langle \left( F_e / \hat{F} \right)^2 \right\rangle^\beta - b K_e + c \exp(-rt), \quad (2)$$

where  $\mathbf{F}_i$  is the  $i$ th fluctuation flow state corresponding to the source term  $\mathbf{S}_i$ ,  $a, b, c$  are parameters of the adaptive dynamics,  $\hat{F}$  is a typical scale of flow,  $r$  is an inverse time scale of decay of the background production term.  $K_e$  is the conductivity of edge  $e$  and  $F_e$  is the flow through edge  $e$ . The angle brackets denote an average over the contributions from all different fluctuating states. Finally, we assume that there is a typical scale  $\hat{S}$  for the source strengths.

We choose the following nondimensionalization:

$$\begin{aligned} K &= \frac{a}{b} (\hat{S} / \hat{F})^{2\beta} \tilde{K}, \quad t = \frac{1}{b} \tilde{t}, \quad \mathbf{F} = \hat{S} \tilde{\mathbf{F}} \\ L &= \hat{L} \tilde{L}, \quad \mathbf{S} = \hat{S} \tilde{\mathbf{S}}. \end{aligned} \quad (3)$$

The definitions of the symbols follow the main paper:  $K$  is the vessel conductivity,  $t$  is time,  $\mathbf{F}$  is the current vector,  $L$  is the vessel length, and  $\mathbf{S}$  is the source strength. Quantities with a tilde are dimensionless and quantities with a hat are typical scales. The model equations then reduce to the dimensionless system

$$\tilde{\mathbf{F}} = \tilde{K} \tilde{L}^{-1} \Delta (\Delta^T \tilde{K} \tilde{L}^{-1} \Delta)^\dagger \tilde{\mathbf{S}} \quad (4)$$

$$\frac{d\tilde{K}_e}{d\tilde{t}} = \langle \tilde{F}_e^2 \rangle^\beta - \tilde{K}_e + \kappa \exp(-\tilde{t}/\rho), \quad (5)$$

with the dimensionless control parameters  $\kappa = (c/a)(\hat{F}/\hat{S})^{2\beta}$ ,  $\rho = b/r$ .

## II. RESULTS FOR OTHER BOUNDARY CONDITIONS AND LATTICES

In this section we show computational results for other lattices, boundary conditions, and fluctuation functions. In all cases, we use the same parameter values as in the main paper.

### A. Gaussian fluctuations with a source at the left side

Here, we show results for Gaussian collective fluctuations where the source is located at the left side of the network. This models the situation for leaf embryos. Gaussian fluctuations are given by

$$f(x) = e^{-\frac{x^2}{2\sigma}}. \quad (6)$$

---

\* henrikr@sas.upenn.edu

† katifori@sas.upenn.edu

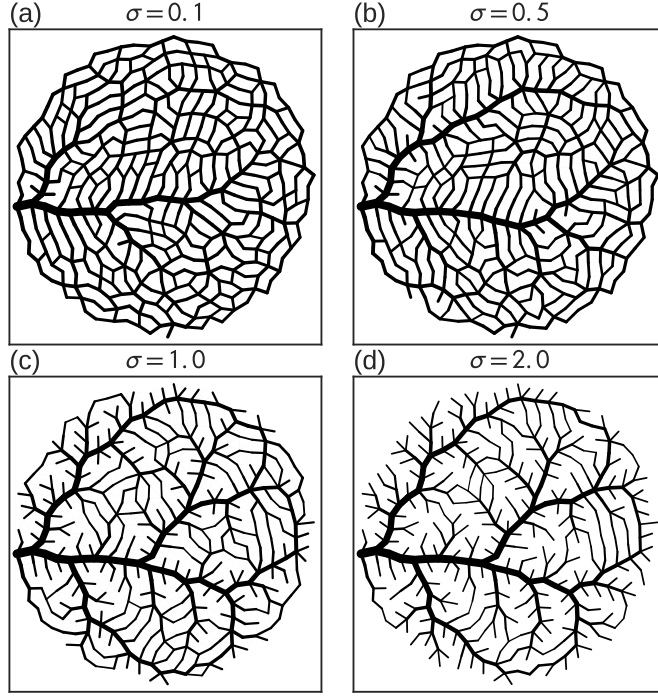

FIG. 1. Network topologies with Gaussian distributed collective fluctuations and a source on the left of the network, modeling a leaf embryo.

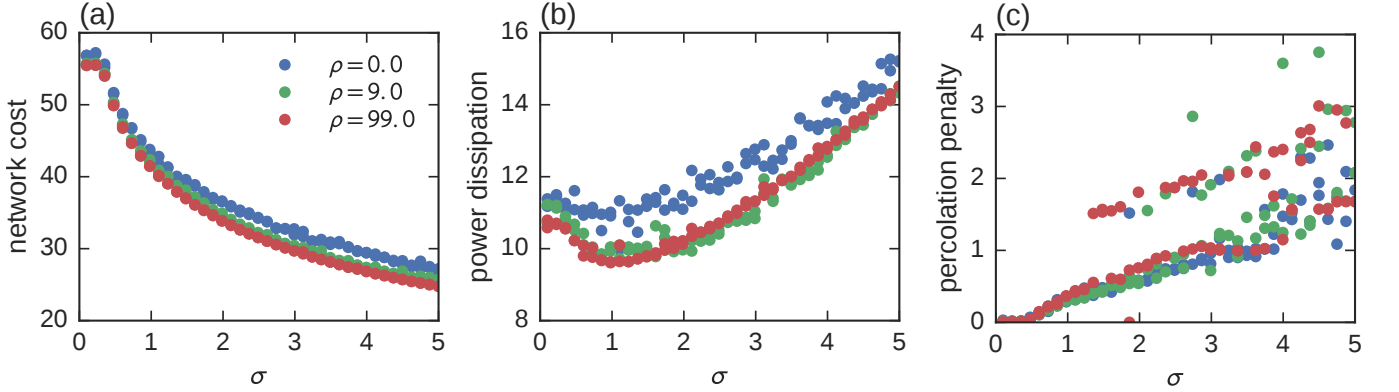

FIG. 2. Network phenotypes as a function of the correlation length for Gaussian distributed collective fluctuations and a source on the left of the network, modeling a leaf embryo. The second branch in (c) corresponds to networks where the source is only connected to the source through a single edge.

The network phenotypes show the same qualitative behavior as for the case of the main paper, where the source was at the center. The one exception is the percolation penalty (Fig. 2c), which shows two branches. This is because as  $\sigma$  increases and the number of loops decreases, it becomes more likely that the source is only connected by a single edge to the rest of the network. In contrast, with the source in the center, this is unlikely to happen. This branching can also be seen in the phenotypic space (Fig. 3).

We note that in this supplement, the percolation penalty is defined as

$$A = \sum_e \frac{A_e}{A_{tot}}, \quad (7)$$

in contrast to the main paper, where we additionally divided by the number of edges.

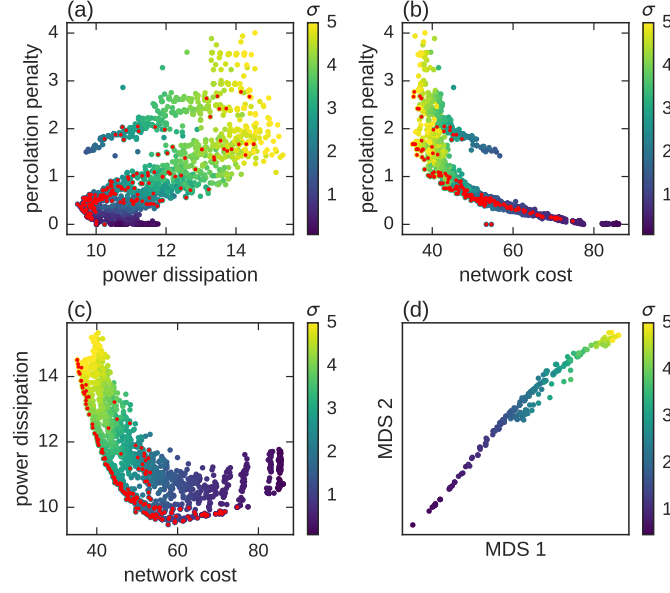

FIG. 3. Phenotypic space of networks with Gaussian distributed collective fluctuations and a source on the left of the network, modeling a leaf embryo. The second branch seen in panels (a) and (b) corresponds to networks where the source is connected to the rest of the network by a single edge, which is highly vulnerable to damage.

### B. Exponential fluctuations

In this subsection we show results for exponentially distributed collective fluctuations,

$$f(x) = e^{-\frac{x}{\sigma}}. \quad (8)$$

We find no qualitative difference between exponential and Gaussian distributed sources in the phenotypes as a function of  $\sigma$  or the phenotypic space. The results are shown in Figs. 4, 5, 6, 7, 8 for sources at the left side and in the center of the network.

### C. Random fluctuations

In this subsection we show results from random fluctuations. We consider fluctuating states

$$(S_i)_j = \begin{cases} -k & \text{with probability } p \\ 0 & \text{with probability } 1 - p \end{cases} \quad (9)$$

for  $j = 1, \dots, N - 1$ . The source is normalized to  $(S_i)_0 = \sum_{j>0} (S_i)_j = 1$ . This normalization sets the value of the constant  $k$ . In the case of these random fluctuations, we consider fluctuation averages over 100 different arrangements of the sources that all satisfy the above probabilistic condition. For these types of fluctuations, the resulting network often does not connect each node in the original lattice to the sink node. Thus, our metrics such as the percolation penalty, network cost, and uniform energy cannot be directly compared anymore. Yet, inspecting the simulation results for various values of  $p$  shows that this model does not reproduce hierarchically ordered networks, see Fig. 9 and Fig. 10. Instead, randomly positions fluctuations produce networks similar to those obtained from collective fluctuations for small fluctuation length scales  $\sigma$ . Varying the probability of switching nodes on or off appears to simply change the density of loops.

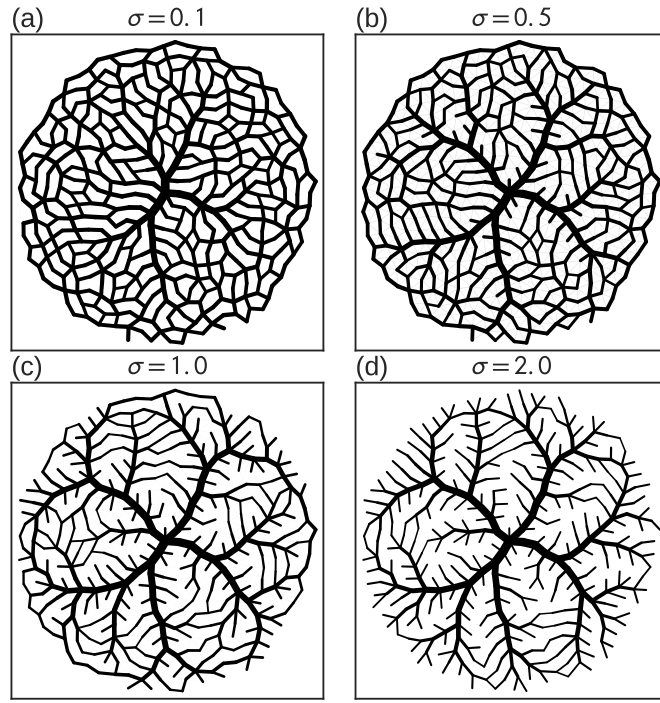

FIG. 4. Network topologies with exponentially distributed collective fluctuations. The networks resemble those produced using Gaussian collective fluctuations (shown in the main paper).

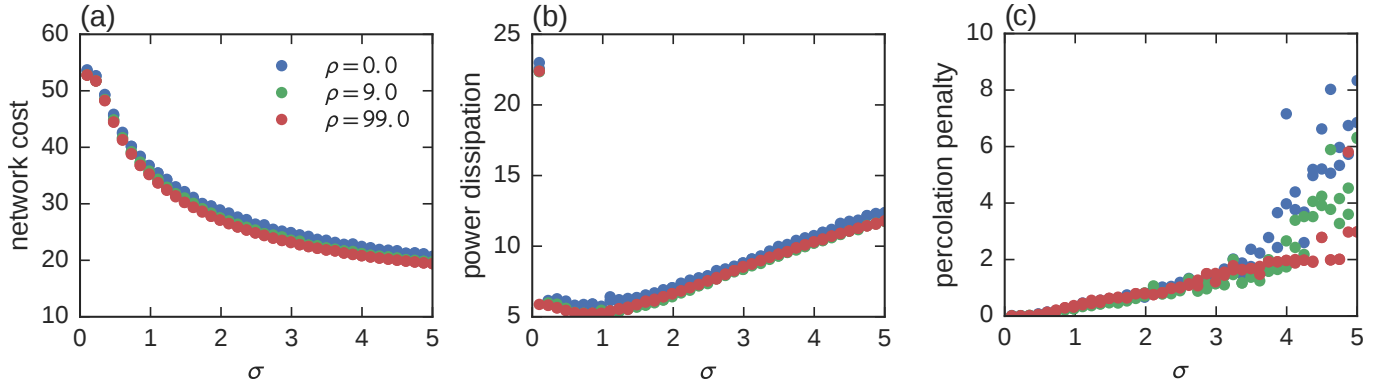

FIG. 5. Dependence of network phenotypes on correlation length for exponentially distributed collective fluctuations with one source at the center. The phenotypes are comparable to those found using Gaussian fluctuations, as shown in the main paper.

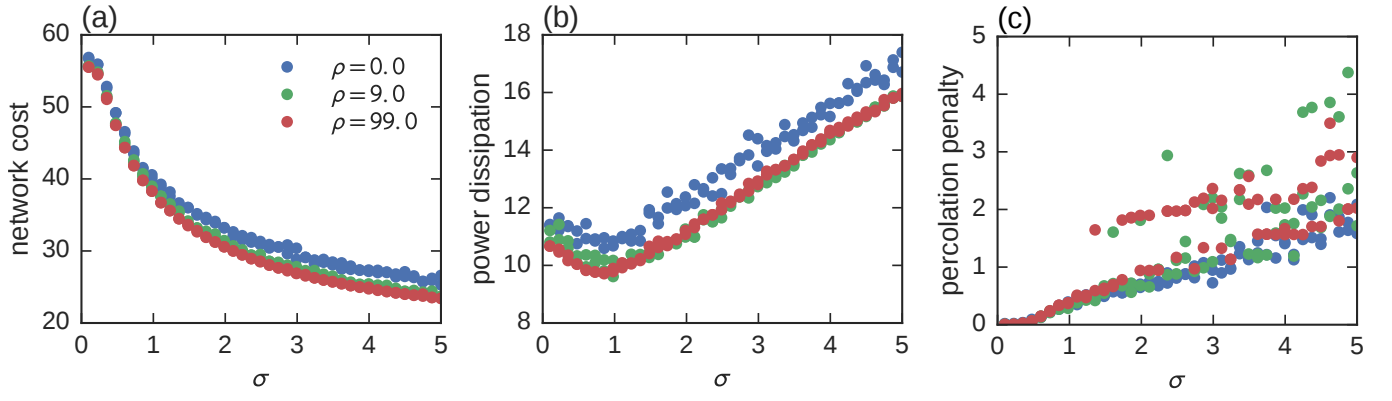

FIG. 6. Dependence of network phenotypes on correlation length for exponentially distributed collective fluctuations with one source at the left boundary. Two distinct phases can be discerned in the percolation penalty. These are due to the source node being connected to the rest of the network by one edge. Thus, removing that edge leads to a very large value of the penalty.

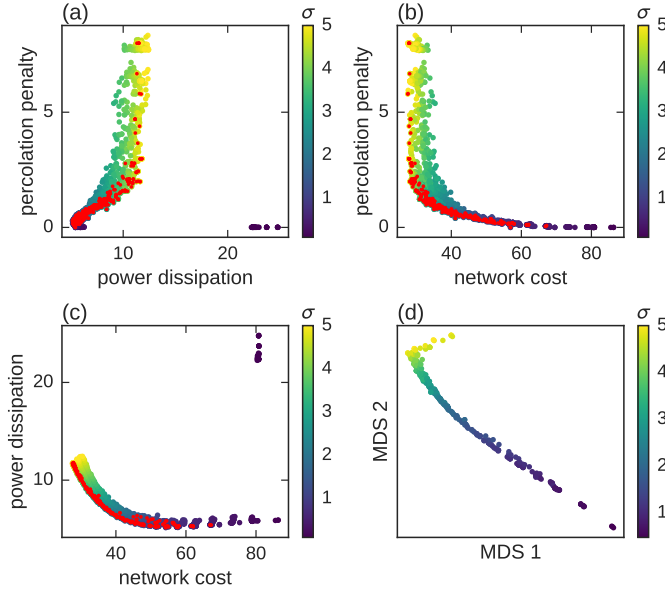

FIG. 7. Phenotypic space for exponentially distributed collective fluctuations with one source at the center. The space is comparable to that found using Gaussian fluctuations as in the main paper.

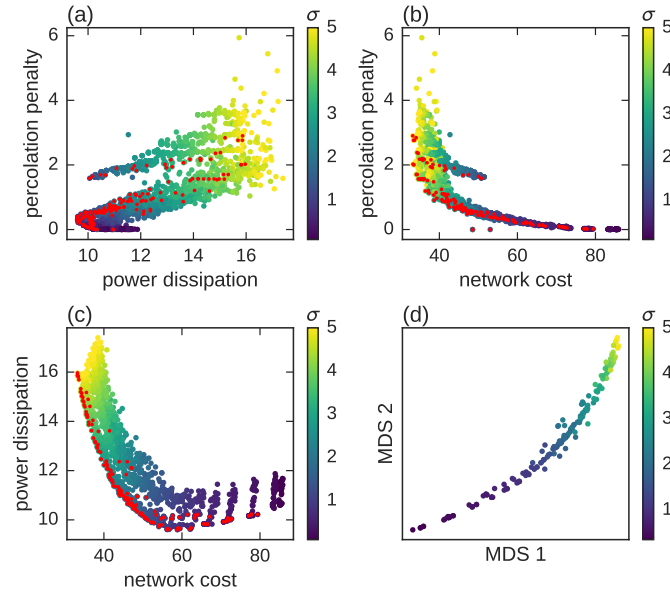

FIG. 8. Phenotypic space for exponentially distributed collective fluctuations with one source at the left boundary. In the percolation penalty there are two distinct branches that are due to the source node being connected to the rest of the network by only one single edge.

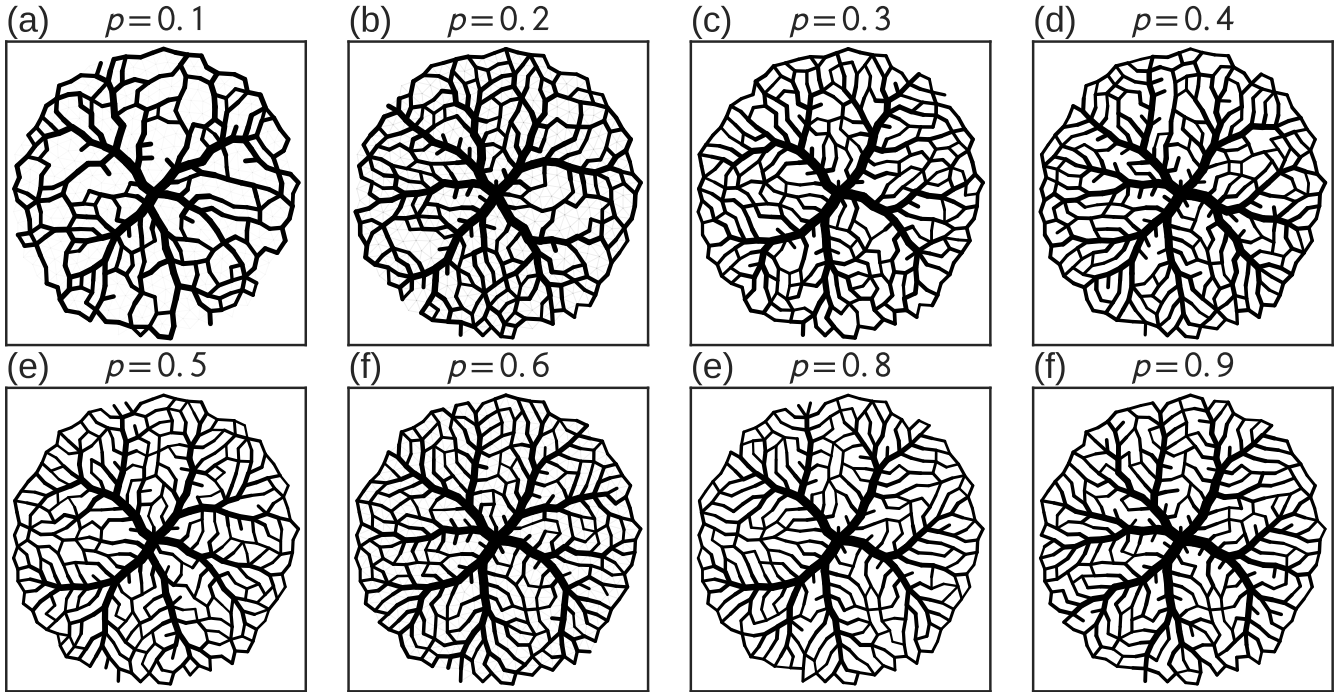

FIG. 9. Random networks for a source at the center and various probabilities  $p$  of any node being a source. The networks show main and secondary veins but no further hierarchical organization. We used parameter values  $\kappa = 1$ ,  $\rho = 99$ .

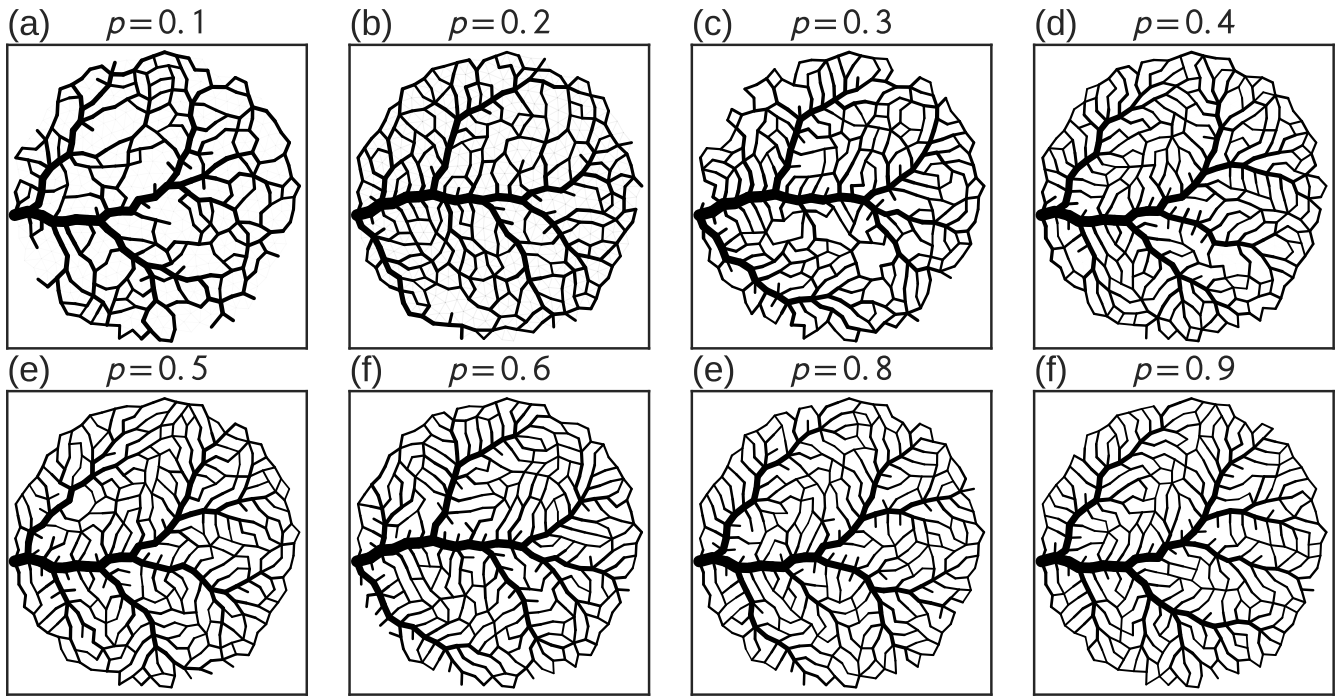

FIG. 10. Random networks for a source at the left boundary and various probabilities  $p$  of any node being a source. The networks show main and secondary veins but no further hierarchical organization. We used parameter values  $\kappa = 1$ ,  $\rho = 99$ .
